# Supplementary material for: Measurement of spin dynamics in a layered nickelate using x-ray photon correlation spectroscopy: Evidence for intrinsic destabilization of incommensurate stripes at low temperatures
Source: arXiv:1912.07306 source file (2021-05-27)
Supplement: Supplementary file 1 [file LSNO-XPCS-Supplemental-Material.pdf]

# Measurement of spin dynamics in a layered nickelate using x-ray photon correlation spectroscopy: Evidence for intrinsic spatial and temporal destabilization of incommensurate stripes at low temperatures
## - Supplemental Material -

Alessandro Ricci, Nicola Poccia, Gaetano Campi, Shrawan Mishra, Leonard Müller, Boby Joseph, Bo Shi, Alexey Zozulya, Marcel Buchholz, Christoph Trabant, James C. T. Lee, Jens Viefhaus, Jeroen B. Goedkoop, Agustinus Agung Nugroho, Markus Braden, Sujoy Roy, Michael Sprung, and Christian Schüßler-Langeheine

(Dated: April 30, 2021)

## SAMPLE PREPARATION

Single-crystalline $La_{1.72}Sr_{0.28}NiO_4$ was grown using floating zone technique. The seed and feed rods were prepared from polycrystalline powder obtained by solid-state reaction of $La_2O_3$, $SrCO_3$ and NiO with an excess of NiO. The reaction was performed at 1200 °C for 20 h with intermediate grinding. Afterwards, the rods were densified at 1500 °C for 5 h. All of the synthesis was carried out in air. Two pieces were cut from the same single crystal, one with (102) and one with (100) surface orientation. Both were lapped with boron carbide powder and polished with alumina suspension. The data presented in Fig. 1 and S2 were taken from the (102)-oriented piece, all other data from the (100)-oriented one.

## ACQUISITION AND ANALYSIS OF STATIC DATA

Static resonant soft x-ray diffraction data were recorded using the ultrahigh-vacuum (UHV) diffractometer designed and constructed at Cologne University. The experiment was performed at the soft X-ray beamline P04 of PETRA III at DESY (Hamburg). At the time of the experiment the beamline provided a photon flux in the order of $10^{12}$ photons/s into a spot of $(v \times h) \approx 50 \times 500\ \mu\text{m}^2$. The x-ray polarization was circular. The peak intensity was detected with an in-vacuum CCD camera placed 0.14 m from the sample. Q-space mapping was done using the xrayutilities package [1].

## ACQUISITION AND ANALYSIS OF XPCS DATA

X-ray photon correlation spectroscopy (XPCS) measurements were carried out at beamline 12.0.2 of the Advanced Light Source at Lawrence Berkeley National Laboratory (USA). The experiment was conducted in a $\theta$-$2\theta$ reflection geometry. Tuning the energy of the incoming linear $\sigma$ polarized x-ray to the $L_3$-edge of Ni (852 eV) yields magnetic sensitivity. The transverse coherence of the beam was established by placing a 5 $\mu$m pinhole approximately 3 mm in front of the sample. The photon flux on the sample in this setting was about $10^9$ ph/s. A CCD placed 0.45 m away served as detector. We took a series of images with an integration time of 10 s each. The readout time of the CCD in between to images was 1 s, such that the time delay between two images [$\Delta t$ in Fig. 2(a)] was 11 s. For the XPCS analysis we used a $q$-space range symmetric to the peak center [see red frame in Fig. 2(a)].

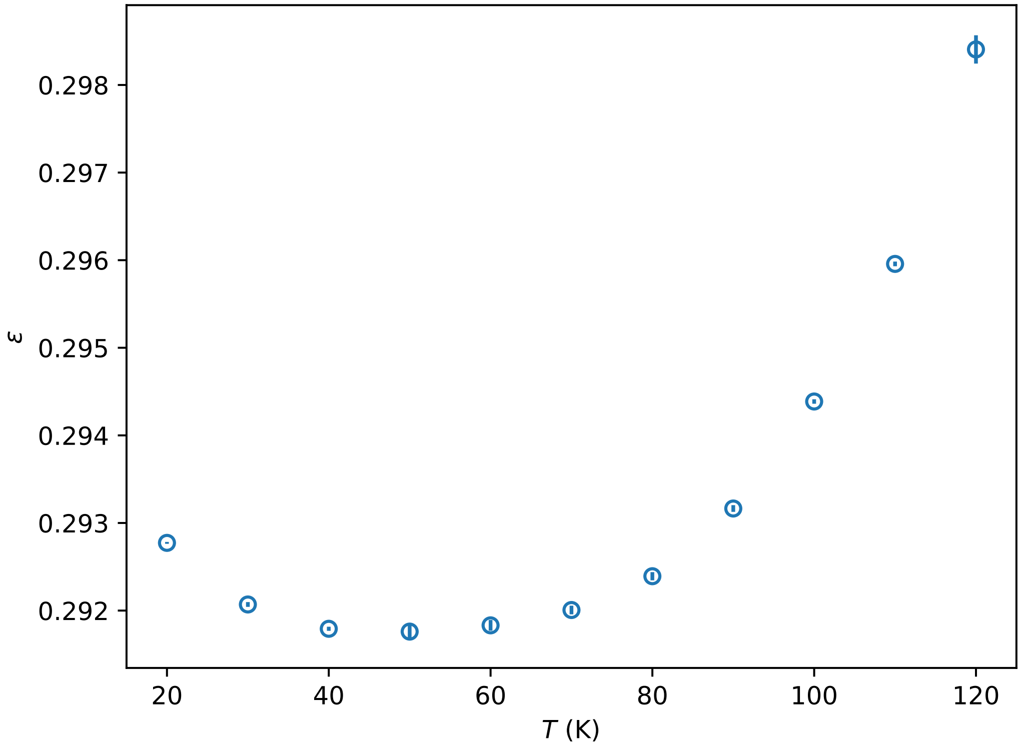


FIG. S1. Temperature dependence of the incommensurability parameter $\epsilon$ determined from the H-position of the spin-order peak [cf. Fig.1(a)].

Its extension is approximately $\pm 0.0024$ r.l.u. along K (vertical direction on the detector); along the horizontal direction H and L extend approximately linearly from $-0.0008$ r.l.u. along H and $-0.0053$ r.l.u. along L to $+0.0008$ r.l.u. along H and $+0.0053$ r.l.u. along L relative to the peak center. The H-position was adjusted to follow the peak shift with temperature.

## TEMPERATURE DEPENDENCE OF $\epsilon$

As seen in other studies for doping levels below 1/3, the incommensurability parameter $\epsilon$ changes towards the commensurate value 1/3 not only at high but also at low temperatures (Fig. S2). These values were determined from the SO peak position [Fig. 1(a)]. The CO peak (see below) shows the same trend. Quantitatively the $\epsilon$-values we determine from SO and CO deviate by about 1 percent ($\delta\epsilon \approx 0.0023$), which we assign to residual misalignment in our setup.

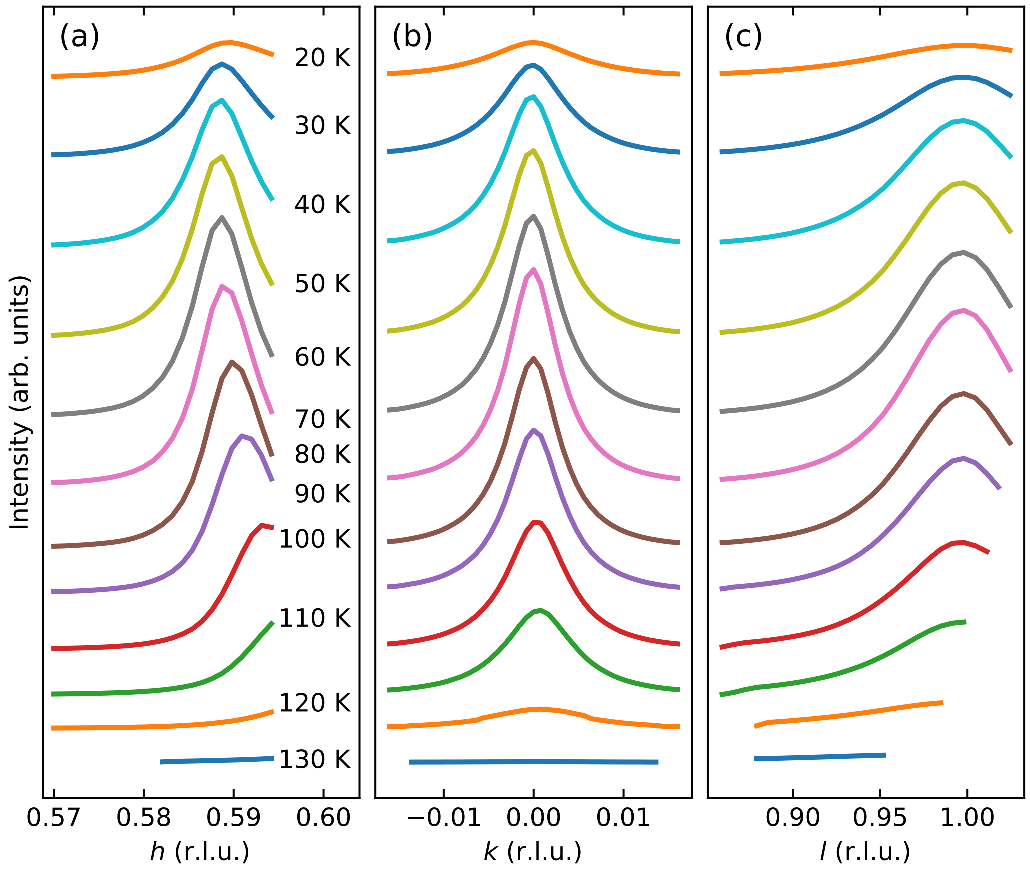


FIG. S2. Static data from the charge order. (a-c) are line cuts along different reciprocal space directions though the charge order peak at different sample temperatures corresponding to those through the spin order peak in Fig. 1(a-c).

## CHARGE STRIPE ORDER

Like the spin peak studied in detail, also the charge stripe peak shows a broadening and loss of intensity upon cooling (Fig. S2). Because of the temperature dependence of $\epsilon$, the peak moves out of the Ewald sphere of the experiment for high and low temperatures.

[1] D. Kriegner, E. Wintersberger, and J. Stangl, xrayutilities: a versatile tool for reciprocal space conversion of scattering data recorded with linear and area detectors, J. Appl. Cryst. **46**, 1162 (2013).
